# Supplementary material for: Temperature-Dependent Electron-Electron Interaction in Graphene on SrTiO3
Source: arXiv:1710.03917 source file (2017-10-11)
Supplement: Supplementary file 1 [file Supplementary_final.pdf]

Supplementary Information for

# Temperature-dependent electron-electron interaction in graphene on $SrTiO_3$

Hyejin Ryu, Jinwoong Hwang, Debin Wang, Ankit S. Disa, Jonathan Denlinger, Yuegang Zhang, Sung-Kwan Mo*, Choongyu Hwang*, and Alessandra Lanzara

*Email: SKMO@lbl.gov; ckhwang@pusan.ac.kr*

## 1. The electron band structure of graphene/$SrTiO_3$

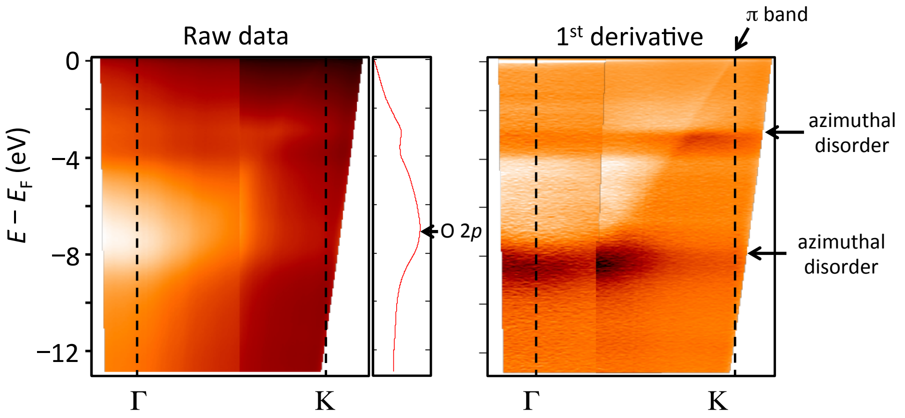


**Figure S1**. An ARPES intensity map of graphene/$SrTiO_3$.

As shown in Fig. S1, the electron band structure of $SrTiO_3$ is not observed except an O 2*p* atomic level observed at ≈7 eV below Fermi energy[1]. The non-dispersive states observed at ≈3 eV and ≈8 eV below Fermi energy are observed due to the azimuthal disorder of CVD graphene similar to the highly oriented pyrolytic graphite[2].

## 2. The electron self-energy of graphene/$SrTiO_3$ as a function of temperature

To investigate the temperature-dependent spectral change in more detail, the electron self-energy was taken at several different temperatures as shown in Fig. S2 and compared with the fitting result (black dashed curve) for 180 K data taken from Fig. 3(b) of the main text. At 120 K, the $|E(k) - E_{LDA}(k)|$ dispersion starts to decrease as denoted by red arrows. This self-energy change becomes prominent upon further decreasing temperature especially below $k_x$≈1.65 Å$^{-1}$.

The strong change at higher energy can be attributed to several possible origins, such as hybridization with the oxygen vacancy states[3], dielectric screening by a substrate[4], and strong electron-electron interactions[5]. When the $SrTiO_3$ substrate is annealed, oxygen vacancies can be produced[3] with a binding energy of ≈0.6 eV[6], which roughly coincides with the binding energy where the slope in the energy-momentum dispersion of graphene starts

to decrease. However, when there is hybridization between two electron band structures, the energy spectrum becomes discontinuous at the crossing point of the two bands[7], which is not the case of the observed energy spectrum shown in Fig. 2(a). A dielectric substrate can also play an important role on the self-energy change. The temperature at which the change in the self-energy becomes noticeable is ≤120 K as shown in Fig. S2, which bears proximity to the onset temperature of a phase transition of $SrTiO_3$ from cubic to tetragonal structure at 105 K[8,9] and from classical to quantum paraelectric phase at lower temperatures[10,11]. These phase transitions of $SrTiO_3$ are accompanied by a sharp increase in dielectric constant at low temperatures[12]. In typical charge neutral graphene, with decreasing dielectric constant of a substrate, $v_F$ and the deviation from the linear energy spectrum are enhanced implying strong electronic correlations in low dielectric screening regime[7]. In contrast, in graphene on $SrTiO_3$, the curvature of the energy spectrum is enhanced with decreasing temperature, i.e., increasing bulk dielectric constant of the substrate[12], even stronger than the logarithmic correction can describe. This excludes the dielectric screening as the origin of the self-energy change, but instead, indicates that the enhanced deviation from the linearity is beyond what the dielectric screening effect can describe, revealing strong electron-electron interactions in graphene on $SrTiO_3$.

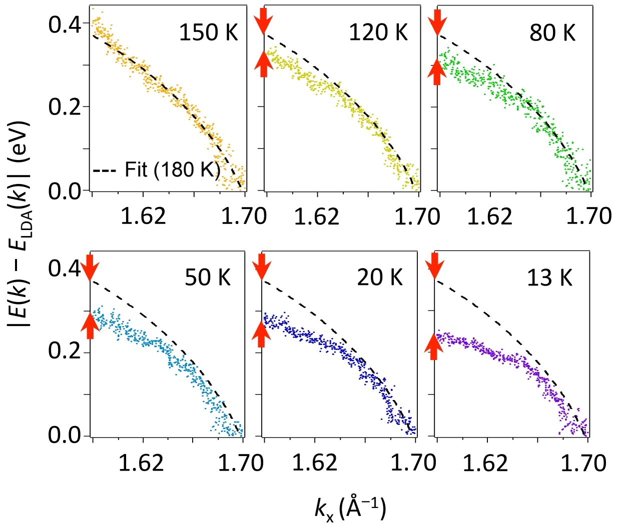


**Figure S2**. $|E(k) - E_{LDA}(k)|$ dispersions at several different temperatures. The black dashed curve is a logarithmic fit to the $|E(k) - E_{LDA}(k)|$ dispersion taken at 180 K for comparison. The red arrows denote the change in electron self-energy at 1.58 $Å^{-1}$.

## 3. An AFM image of $SrTiO_3$

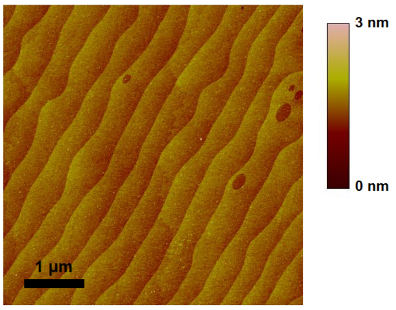


**Figure S3**. An AFM image of an $SrTiO_3(001)$ crystal after thermal treatment with oxygen flow.

## References


1 Aiura, Y.; Hase, I.; Bando, H.; Yasue, T.; Saitoh, T.; Dessau, D. S. *Surf. Sci.* **2002**, *515*, 61.

2 Shou, S. Y.; Gweon, G. –H.; Spataru, C. D.; Graf, J.; Lee, D. –H.; Louie, S. G.; Lanzara, A. *Phys. Rev. B* **2005**, *71*, 161403(R).

3 Zvanut, M. E.; Jeddy, S.; Towett, E.; Janowski, G. M.; Brooks, C.; Schlom, D. *J. Appl. Phys.* **2008**, *104*, 064122.

4 Hwang, C.; Siegel, D. A.; Mo, S. –K.; Regan, W.; Ismach, A.; Zhang, Y.; Zettl, A.; Lanzara, A. *Sci. Rep.* **2012**, *2*, 590.

5 González, J.; Guinea, F.; Vozmediano, M. A. H. *Nucl. Phys. B* **1994**, *424*, 595.

6 Gryaznov, D.; Blokhin, E.; Sorokine, A.; Kotomin, E. A.; Evarestov, R. A.; Bussmann-Holder, A.; Maier, J. *J. Phys. Chem. C* **2013**, *117*, 13776.

7 Hwang, C.; Kim, D. Y.; Siegel, D. A.; Chan, K. T.; Noffsinger, J.; Fedorov, A. V.; Cohen, M. L.; Johansson, B.; Neaton, J. B.; Lanzara, A. *Phys. Rev. B* **2014**, *90*, 115417.

8 Fleury, P. A.; Scott, J. F.; Worlock, J. M. *Phys. Rev. Lett.* **1968**, *21*, 16.

9 Scott, J. F. *Rev. Mod. Phys.* **1974**, *46*, 83.

10 Lytle, F. W. *J. Appl. Phys.* **1964**, *35*, 2212.

11 Muller, K. A.; Berlinger, W.; Tossati, E. *Z. Phys. B* **1991**, 84, 277.

12 Weaver, H. E. *J. Phys. Chem. Solids* **1959**, *11*, 274.
